# Supplementary material for: SWE-Dev: Building Software Engineering Agents with Training and Inference Scaling
Source: arXiv:2506.07636 source file (2025-06-23)
Supplement: Supplementary file 1 [file appendix.tex]

\appendix
\section{Data Sources}\label{app:data_source}
The dataset is constructed from a wide range of visual sources to ensure diversity in content, visual styles, and task scenarios. Below is the full list of data sources used in the dataset, along with a brief description of their contributions:

\begin{itemize}
    \item \textbf{EPIC-KITCHENS \cite{Damen2018EPICKITCHENS}:} This large-scale egocentric vision dataset provides daily activity scenes captured from head-mounted cameras in kitchen environments. It contributes high-quality egocentric views with natural object interactions.
    \item \textbf{Sina Weibo:} Social media content from Weibo adds dynamic and culturally specific imagery, including real-life and staged scenes.
    \item \textbf{Taobao:} E-commerce images from Taobao provide diverse commercial imagery, focusing on structured object arrangements and product displays.
    \item \textbf{Baidu Images:} This large-scale image search platform contributes a variety of general-purpose images with a focus on Chinese content.
    \item \textbf{Xiaohongshu:} Lifestyle images from Xiaohongshu add visually appealing compositions and diverse object arrangements.
    \item \textbf{500px:} High-quality professional photography from 500px introduces artistic compositions and complex scenes.
    \item \textbf{Google Images:} A general-purpose image search platform that contributes a wide variety of visual contexts, ensuring global diversity.
    \item \textbf{Personal Photography:} Custom photographs taken by the authors provide unique, controlled scenes tailored to specific reasoning tasks.
    \item \textbf{SheTu:} Licensed stock photos from shetu add professionally curated content with diverse object arrangements and scenarios.
\end{itemize}

The combination of these sources enables the dataset to cover a broad range of scenarios, from everyday activities to artistic and staged environments. This diversity ensures that the dataset is representative of real-world visual reasoning challenges.

\section{Experiment Setup}

\subsection{Prompt Modifications}
\label{app:prompt-few-shot}
In our experiments, we utilized the InternVL3-8b model as our base model. To evaluate the impact of different prompting strategies on VLMs, we conducted three sets of experiments using identical datasets but varying prompt approaches.

\textbf{Experimental Design}

\begin{itemize}
    \item \textbf{Direct Sampling:} Basic inference without additional context or examples
    \item \textbf{Few-Shot Learning:} Including task-specific examples in the prompt
    \item \textbf{Two-Stage Prompting:} Incorporating image caption generation before task-specific questions
\end{itemize}

This comparative study aims to quantify the influence of different prompting strategies on VLM performance, maintaining consistent model parameters and datasets across all experiments to isolate the effect of prompt engineering.

\begin{tcolorbox}[
    colback=white,
    colframe=prompt-color,
    coltitle=black,
    title=\textbf{Two-Stage Prompting Strategy},
    fonttitle=\bfseries,
    arc=2mm,
    fontupper=\footnotesize,
    breakable,
    enhanced,
    coltitle=black
]

\textbf{Stage 1: Image Caption Generation}

\begin{tcolorbox}[
    colback=gray!10,
    colframe=black!50,
    title=\textbf{CAPTION PROMPT},
    fonttitle=\bfseries,
    arc=2mm,
    fontupper=\small,
    enhanced,
    breakable
]

\begin{verbatim}
Please describe what you see in this image.

Example Response:

{
    "image_caption": "The image depicts a Japanese dining setting 
     with multiple dishes arranged on a table. The scene includes:

    1. Main Course (Foreground)
       • Donburi-style bowl with tonkatsu rice
       • Topped with shredded egg (kinshi tamago)
       • Garnished with finely chopped green onions

    2. Side Dishes
       • Sushi plate: Three pieces on decorative seaweed base
       • Harumaki (spring rolls): Vegetable-filled, sesame-garnished
       • Tempura or katsu: Breaded and fried, with drizzled sauce

    3. Tea Service
       • Traditional ceramic teapot: Blue and white pattern
       • Two matching teacups with geometric designs

    4. Additional Items
       • Background bowl: Secondary rice dish or soup
       • Side plate: Stir-fried vegetables with meat

    5. Condiments
       • Small ceramic pitcher containing soy sauce

    Overall Ambiance: The presentation suggests an authentic Japanese 
    restaurant setting, with attention to traditional serving methods 
    and aesthetic arrangement."
}
\end{verbatim}

\end{tcolorbox}

\textbf{Stage 2: Task-Specific Questions}

\textbf{a. Spatial Relation Task}

\begin{tcolorbox}[
    colback=gray!10,
    colframe=black!50,
    title=\textbf{RELATION BASE PROMPT},
    fonttitle=\bfseries,
    arc=2mm,
    fontupper=\small,
    enhanced,
    breakable
]

\begin{verbatim}
You should output a json string with format {"answer": "str"} 
where str must be one of ["up", "under", "back", "front", "left", "right"]
Your output should be directly parsed by json.loads function
eg.json{"answer": "left"}
Now the question is:
\end{verbatim}
\end{tcolorbox}

\textbf{b. Counting Task}

\begin{tcolorbox}[
    colback=gray!10,
    colframe=black!50,
    title=\textbf{COUNTING BASE PROMPT},
    fonttitle=\bfseries,
    arc=2mm,
    fontupper=\small,
    enhanced,
    breakable
]

\begin{verbatim}
You should output a json string with format {"answer": a int number}
Your output should be directly parsed by json.loads function 
eg.json{"answer": 1}
Now the question is:
\end{verbatim}

\end{tcolorbox}

\end{tcolorbox}

\begin{tcolorbox}[
    colback=white,
    colframe=prompt-color,
    coltitle=black,
    title=\textbf{Task-Specific Examples},
    fonttitle=\bfseries,
    arc=2mm,
    fontupper=\footnotesize,
    breakable,
    enhanced,
    coltitle=black
]

\textbf{Counting Task Examples}

\begin{tcolorbox}[
    colback=gray!10,
    colframe=black!50,
    title=\textbf{COUNTING BASE PROMPT EXAMPLES},
    fonttitle=\bfseries,
    arc=2mm,
    fontupper=\small,
    enhanced,
    breakable
]

\begin{verbatim}
You should output a json string with format {"answer": a int number}. 
Your output should be directly parsed by json.loads function.

Here are some examples:
Q: How many dogs are in the image?
A: json{"answer": 2}

Q: Count the number of red apples on the table.
A: json{"answer": 5}

Q: How many people are wearing glasses in this photo?
A: json{"answer": 3}

Invalid answers:
- json{"answer": "three"} (answer must be integer, not string)
- json{"answer": 2.5} (answer must be integer, not float)
- "2" (must be valid json format)

Now the question is:
\end{verbatim}

\end{tcolorbox}

\textbf{Spatial Relation Task Examples}

\begin{tcolorbox}[
    colback=gray!10,
    colframe=black!50,
    title=\textbf{RELATION BASE PROMPT EXAMPLES},
    fonttitle=\bfseries,
    arc=2mm,
    fontupper=\small,
    enhanced,
    breakable
]

\begin{verbatim}
You should output a json string with format {"answer": "str"}
where str must be one of ["up", "under", "back", "front", "left", "right"]
Your output should be directly parsed by json.loads function

Here are some examples:
Q: What is the spatial relation between the cat and the table? 
A: json{"answer": "under"}

Q: Where is the lamp relative to the desk? 
A: json{"answer": "up"}

Q: What is the position of the car relative to the building? 
A: json{"answer": "front"}

Invalid answers:
- json{"answer": "below"} (must use "under" instead)
- json{"answer": "on"} (not in valid relation list)
- "left" (must be valid json format)

Now the question is:

VALID_RELATIONS = ["up", "under", "back", "front", "left", "right"]
\end{verbatim}
\end{tcolorbox}

\end{tcolorbox}

\subsection{Image Augmentation}\label{app:augmentation}
To probe the perceptual robustness of vision–language models, we expose each
image to two \emph{complementary} categories of perturbations:

\begin{enumerate}[leftmargin=1.4em,label=\textbf{\arabic*.}]
    \item \textbf{Geometric Flip.}
          We apply \emph{horizontal} (`left–right'') and
          \emph{vertical} (`top–bottom'') flips\footnote{Implemented with
          \texttt{PIL.Image.transpose}. The operation leaves low-level statistics
          unchanged while altering global object layout.} to examine whether
          models properly internalise spatial relations rather than memorising
          canonical arrangements.

    \item \textbf{Noise Injection.} %
          For each sample we \emph{randomly pick one} of the following four
          photometric corruptions:
          \begin{itemize}[leftmargin=1.2em]
              \item \textbf{Gaussian Noise} — additive noise drawn from
                    $\mathcal{N}(0,\sigma^{2})$ with $\sigma=15$
                    (RGB range $[0,255]$), simulating sensor noise;
              \item \textbf{Salt-and-Pepper Noise} — $2\%$ of pixels are
                    randomly set to either 0 or 255, creating high-contrast
                    outliers;
              \item \textbf{Gaussian Blur} — convolution with a $5{\times}5$
                    kernel and $\sigma_{\mathrm{blur}}=1.5$, softening edges;
              \item \textbf{Contrast/Brightness Shift} — linear transform
                    $I'=\alpha I+\beta$ with $\alpha\!\sim\!\mathcal{U}(0.8,1.2)$
                    and $\beta\!\sim\!\mathcal{U}(-20,20)$, altering global
                    luminance.
          \end{itemize}
\end{enumerate}

\paragraph{Illustrative Cases.}
We accompany the augmentation protocol with two representative examples.  
Case~1 in Figure~\ref{fig:aug_case1} and Case~2 in Figure~\ref{fig:aug_case2}.

\begin{figure*}[t]
    \centering
    \includegraphics[width=\linewidth]{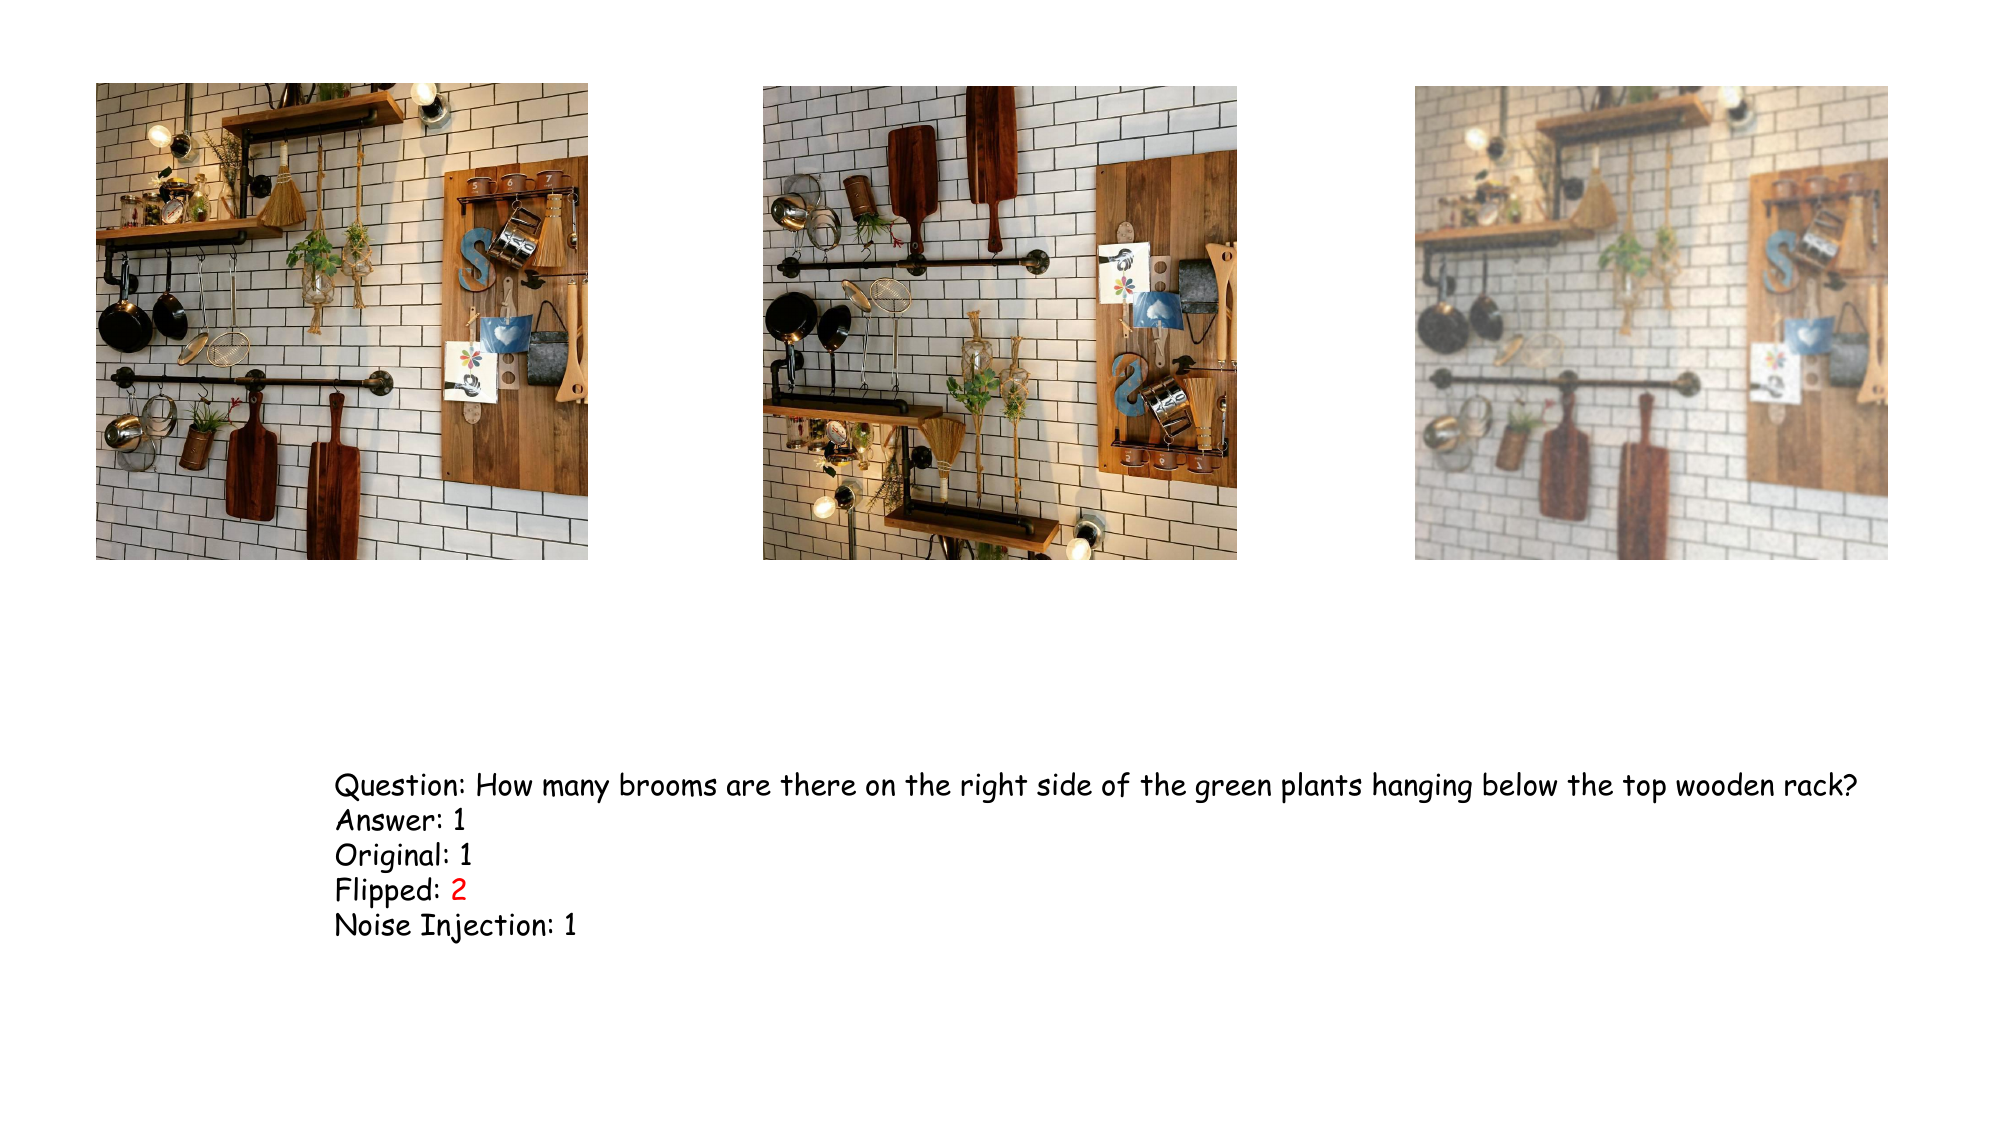}
    \vspace{-4em}
    \caption{\textbf{Augmentation Case~1.}
             \textit{Left}: original kitchen scene.
             \textit{Centre}: horizontally flipped.
             \textit{Right}: Gaussian-blurred and contrast-shifted.
             The query targets the broom count \emph{right} of the hanging
             plants; flipping reverses the reference frame and breaks the
             model’s grounding.}
    \label{fig:aug_case1}
\end{figure*}

\begin{figure*}[t]
    \centering
    \includegraphics[width=\linewidth]{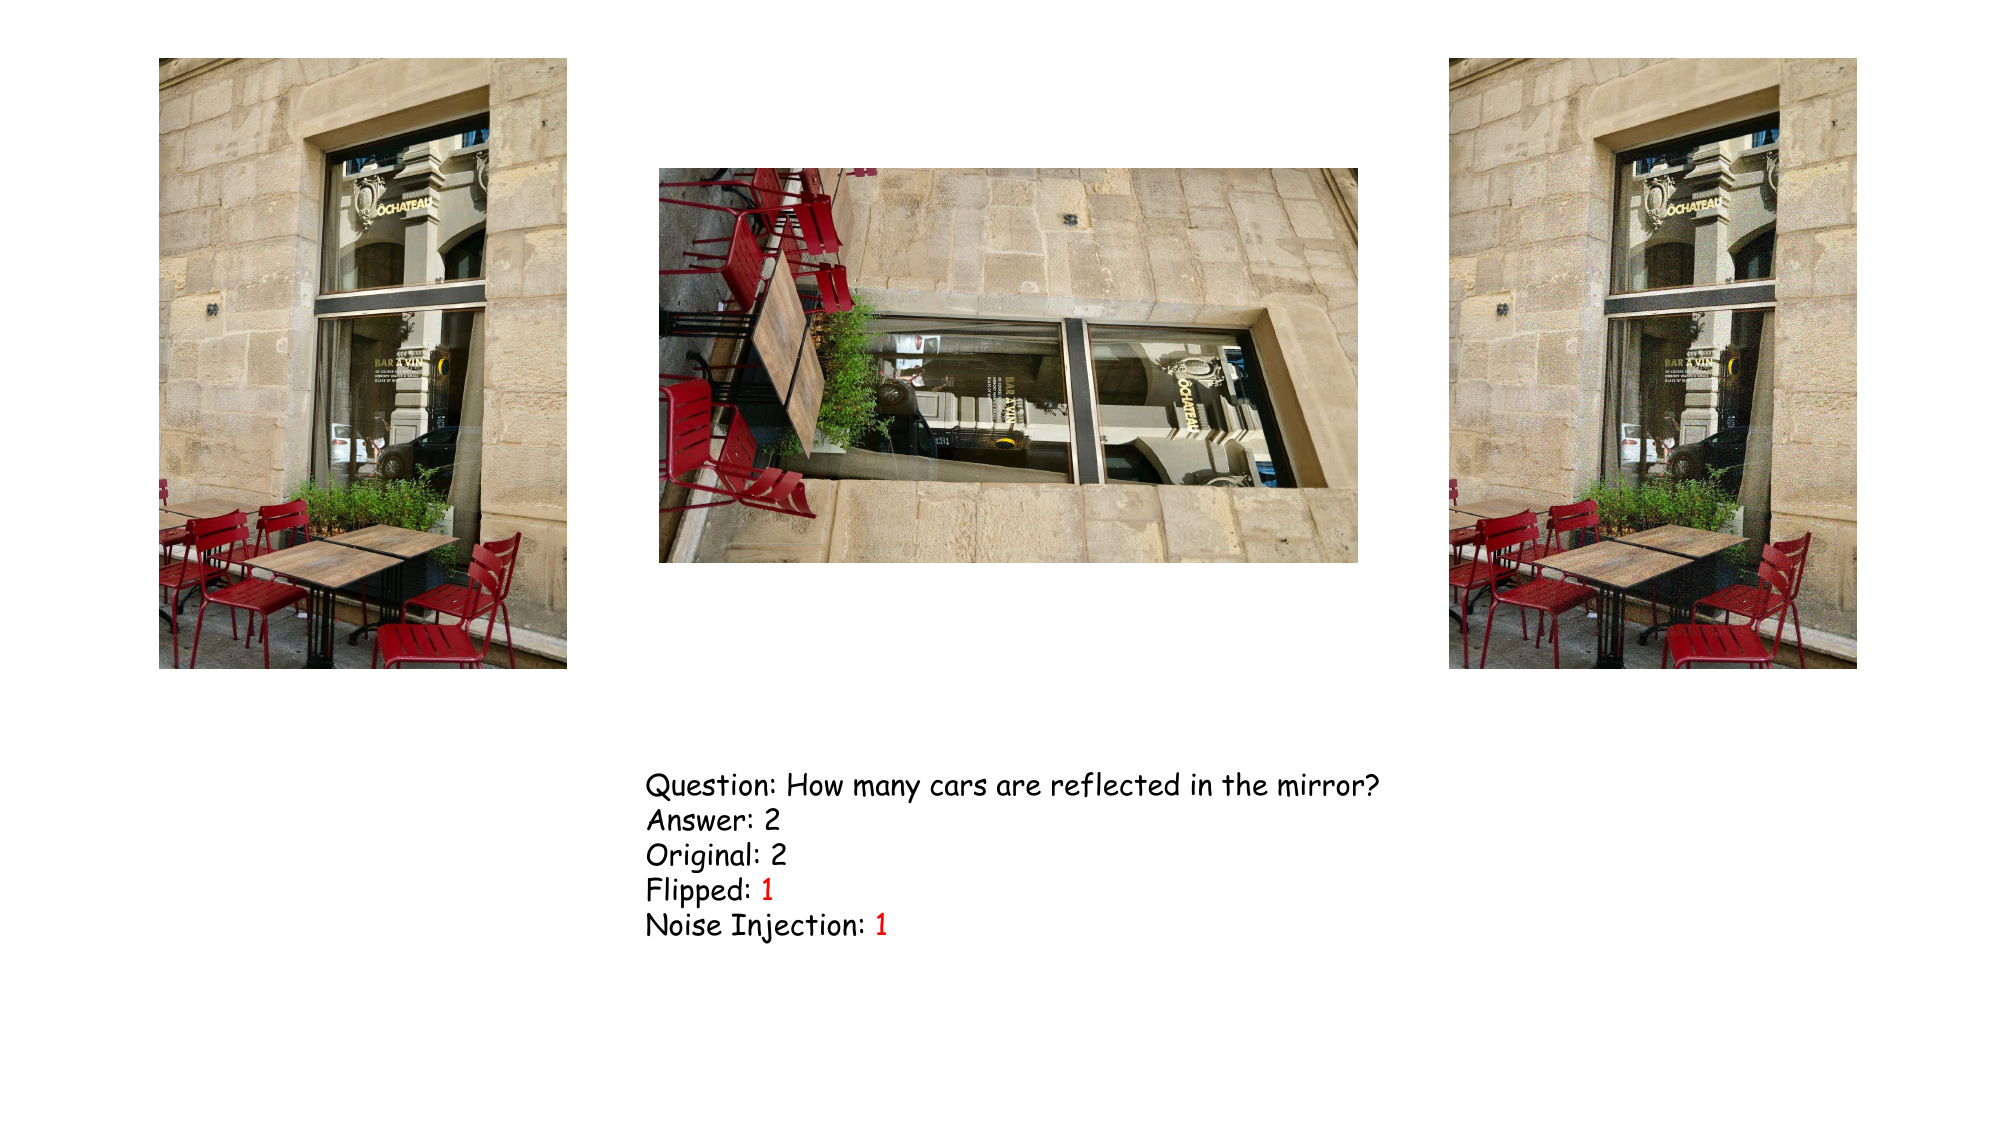}
    \vspace{-4em}
    \caption{\textbf{Augmentation Case~2.}
             Street-side café scene with reflective window.
             Flipping disrupts left–right reflection cues, leading to
             under-counting of cars, while salt-and-pepper noise adds spurious
             edges yet leaves spatial layout intact.}
    \label{fig:aug_case2}
\end{figure*}
